# Supplementary material for: Structural Insights and an IP-based Solution Method for Patient-to-room Assignment under Consideration of Single Room Entitlements
Source: arXiv:2401.00221 source file (2024-02-19)
Supplement: Supplementary file 1 [file 10_Appendix.tex]

\newpage
\appendix 
\section{Appendix}
\subsection{IP with same-day transfers \ref{lp:SDTransfer}} \label{app:lpC}
\beforeMyLP{2}
\begin{maxi!}
{}{(\privobj,  \transobj) \label{C0}}{\label{lp:SDTransfer}}{}
\addConstraint{\sum_{r \in \R} x_{pr}}{= 1\label{C1}}{\forall p \in \P}
\addConstraint{\sum_{p \in \fp(t)} x_{pr} + \sum_{p \in \fp(t) \cap \priv} (c_r-1)s_{prt}}{\le c_rg_{rt}\label{C2}}{\forall t \in \T, r \in \R}
\addConstraint{\sum_{p \in \mp(t)} x_{pr} + \sum_{p \in \mp(t) \cap \priv} (c_r-1)s_{prt}}{\le c_r(1-g_{rt})\label{C3}\:}{\forall t \in \T, r \in \R}
\addConstraint{s_{prt}}{\le x_{pr} \label{C5}}{\forall t \in \T,  r \in \R, p \in \priv}
\addConstraint{x_{pr}+x_{qr}}{\le 1 \label{C6}}{\forall r \in \R, (p,q) \in \conflicts}
\addConstraint{x_{pr},g_{rt},s_{prt}}{\in \{0,1\} \notag{}}{\forall r \in \R, t \in \T, p \in \P.}
\end{maxi!}
\afterMyLP
\subsection{Datasets}\label{app:datasets}

\begin{table}[h!]
    \tiny
    \centering
    \begin{tabular}{|c||c|c|c|c|c||c|c||c||c|}
\hline Instance & Patients & Female & Male & Private & Emergency & $\lor$ & $\los$ & Rooms & Feasible \\\hline
AU01 & 2474 & 1093 & 1381 & 427 & 1173 & 1 & 3 & 16 & True \\
CH01 & 1086 & 495 & 591 & 233 & 312 & 6 & 4 & 14 & True \\
CH02 & 1090 & 445 & 645 & 210 & 294 & 6 & 4 & 14 & True \\
DE01 & 1317 & 726 & 591 & 103 & 423 & 2 & 5 & 13 & True \\
GC01 & 1580 & 653 & 927 & 246 & 266 & 8 & 3 & 14 & True \\
GG01 & 1712 & 1595 & 117 & 235 & 587 & 5 & 3 & 16 & True \\
GG03 & 2995 & 2503 & 492 & 191 & 1826 & 0 & 3 & 18 & False \\
GGKS & 554 & 527 & 27 & 51 & 391 & 0 & 1 & 6 & True \\
HG01 & 870 & 274 & 596 & 51 & 135 & 10 & 2 & 7 & False \\
HG02 & 1938 & 495 & 1443 & 413 & 242 & 7 & 4 & 20 & True \\
HN01 & 804 & 309 & 495 & 127 & 287 & 2 & 3 & 13 & True \\
I1HK$^*$ & 0 & 0 & 0 & 0 & 0 & nan & nan & 5 & True \\
IM02 & 1193 & 419 & 774 & 123 & 341 & 2 & 5 & 20 & True \\
IM08 & 643 & 289 & 354 & 88 & 300 & 1 & 2 & 15 & True \\
IM11 & 1375 & 494 & 881 & 235 & 296 & 3 & 3 & 18 & True \\
IM12 & 1407 & 529 & 878 & 128 & 311 & 4 & 4 & 18 & True \\
IM13 & 1513 & 591 & 922 & 335 & 313 & 4 & 4 & 22 & True \\
IM18 & 1056 & 427 & 629 & 116 & 490 & 1 & 2 & 20 & True \\
IM19 & 741 & 251 & 490 & 109 & 264 & 2 & 1 & 8 & True \\
IM22 & 904 & 413 & 491 & 125 & 384 & 1 & 5 & 19 & True \\
IM31 & 1693 & 766 & 927 & 190 & 739 & 1 & 4 & 20 & True \\
IM32 & 1022 & 416 & 606 & 247 & 437 & 1 & 4 & 14 & True \\
IM33$^*$ & 1 & 0 & 1 & 0 & 1 & 0 & 1 & 1 & True \\
IM42 & 1708 & 754 & 954 & 278 & 1240 & 0 & 5 & 24 & True \\
KI01 & 1025 & 510 & 515 & 179 & 823 & 0 & 2 & 9 & True \\
KI03 & 1152 & 478 & 674 & 186 & 482 & 1 & 2 & 9 & True \\
KI04 & 1328 & 693 & 635 & 146 & 1102 & 0 & 2 & 8 & False \\
KI05 & 960 & 427 & 533 & 29 & 651 & 0 & 4 & 11 & False \\
KI07 & 2126 & 980 & 1146 & 280 & 1822 & 0 & 2 & 15 & True \\
KI08 & 493 & 209 & 284 & 29 & 353 & 0 & 3 & 19 & True \\
KIKU$^*$ & 0 & 0 & 0 & 0 & 0 & nan & nan & 2 & True \\
KIPS & 73 & 40 & 33 & 11 & 60 & 0 & 24 & 10 & True \\
KJ01 & 186 & 114 & 72 & 12 & 78 & 1 & 19 & 12 & True \\
KJ02 & 196 & 146 & 50 & 12 & 105 & 0 & 11 & 8 & True \\
KJ03 & 84 & 81 & 3 & 26 & 31 & 3 & 41 & 7 & True \\
KJEK & 50 & 13 & 37 & 6 & 4 & 13 & 28.5 & 5 & True \\
KK01 & 695 & 327 & 368 & 93 & 241 & 4 & 2 & 7 & True \\
MK01 & 372 & 133 & 239 & 56 & 55 & 7 & 2 & 4 & True \\
NAST & 3745 & 1704 & 2041 & 299 & 3735 & 0 & 1 & 29 & True \\
NC01 & 1816 & 882 & 934 & 331 & 674 & 2 & 4 & 20 & True \\
NE01 & 1041 & 580 & 461 & 45 & 429 & 1 & 2 & 8 & True \\
NE02 & 1682 & 877 & 805 & 411 & 630 & 1 & 3 & 18 & True \\
NE03 & 222 & 93 & 129 & 27 & 158 & 0 & 18 & 8 & True \\
NE07 & 797 & 394 & 403 & 93 & 333 & 1 & 4 & 16 & True \\
NE08 & 315 & 154 & 161 & 37 & 198 & 0 & 4 & 15 & True \\
SG01 & 628 & 318 & 310 & 26 & 253 & 1 & 5 & 8 & True \\
ST01 & 1283 & 573 & 710 & 218 & 674 & 0 & 3 & 20 & True \\
SZT1 & 317 & 139 & 178 & 78 & 227 & 0 & 6 & 12 & True \\
UC01 & 1205 & 517 & 688 & 206 & 437 & 1 & 5 & 16 & True \\
UR01 & 1940 & 493 & 1447 & 402 & 626 & 7 & 3 & 20 & True \\
WEA1 & 234 & 79 & 155 & 27 & 32 & 18 & 17 & 13 & True \\\hline
    \end{tabular}
    \caption{Overview of real world data. Starred instances were excluded for being trivial/empty. For $\lor$ and $\los$ the given values are the medians.}
    \label{tab:instances}
\end{table}
