# Supplementary material for: Structural Insights and an IP-based Solution Method for Patient-to-room Assignment under Consideration of Single Room Entitlements
Source: arXiv:2401.00221 source file (2024-02-19)
Supplement: Supplementary file 2 [file appendix_LPs.tex]

\subsection{IP-formulation without transfers \ref{lp:noTransfer}}\label{sec:IPnoTrans}
In this section, we present an integer programming formulation for PRA without transfers that maximises the number of time periods that private patients spend alone in a room.
We use three sets of binary decision variables: $x_{pr}\in\{0,1\}$, which model whether a patient $p\in \P$ is assigned to a room $r\in \R$ or not, $g_{rt}\in\{0,1\}$, which model whether a female patient is assigned to a room $r\in \R$ in time period $t\in \T$, and $s_{prt}\in\{0,1\}$, which model whether a patient $p \in \P$ is assigned alone to room $r\in \R$ during time period $t\in \T$, i.e.,
\begin{align*}
    x_{pr}&=\begin{cases}
            1,  &\text{if patient }  p \text{ is assigned to room } r \text{ in all time periods } \arr_p\leq t < \dis_p,\\
            0,  &\text{otherwise,}
        \end{cases}\\
    g_{rt} &=\begin{cases}
            1,  &\text{if there is a female patient assigned to room } r \text{ in time period } t,\\
            0,  &\text{otherwise,}
        \end{cases}\\
    s_{prt} &=\begin{cases}
            1,  &\text{if } p \text{ is alone in room } r \text{ in time period } t,\\
            0,  &\text{otherwise.}
        \end{cases}
\end{align*}
We employ the following integer programming formulation \eqref{lp:noTransfer}:
\beforeMyLP{13}
\begin{maxi!}
{}{\privobj = \sum_{t \in \T}\sum_{\substack{p \in \priv(t)}} \sum_{r \in \R}s_{prt}\label{N0}}{\label{lp:noTransfer}}{}
\addConstraint{\sum_{r \in \R} x_{pr}}{= 1\label{N1}}{\forall p \in \P}
\addConstraint{\sum_{p \in \fp(t)} x_{pr} + \sum_{p \in \fp(t) \cap \priv} (c_r-1)s_{prt}}{\le c_rg_{rt}\label{N2}}{\forall t \in \T, r \in \R}
\addConstraint{\sum_{p \in \mp(t)} x_{pr} + \sum_{p \in \mp(t) \cap \priv} (c_r-1)s_{prt}}{\le c_r(1-g_{rt})\label{N3}\:}{\forall t \in \T, r \in \R}
\addConstraint{s_{prt}}{\le x_{pr} \label{N5}}{\forall t \in \T,  r \in \R, p \in \priv}
\addConstraint{x_{pr}+x_{qr}}{\le 1 \label{N6}}{\forall r \in \R, (p,q) \in \conflicts}
\addConstraint{x_{pr}}{= 1 \label{N7}}{\forall (p,r) \in \rpold}
\addConstraint{x_{pr},g_{rt},s_{prt}}{\in \{0,1\} \notag{}}{\forall r \in \R, t \in \T, p \in \P.}
\end{maxi!}
\afterMyLP

Here, we ensure that every patient receives a bed via \eqref{N1}.
Constraints \eqref{N2}, and respectively \eqref{N3}, ensure on the one hand that every double room only contains only either female or male patients up to its capacity, and, on the other hand, they record when a private patient is alone in a double room.
The constraints \eqref{N5} link the single room variables $s_{prt}$ to the patient assignments and \eqref{N6} ensures that all patient conflicts are respected.
Finally, if there exist fixed patient-room assignments, e.g. from previous planning periods that are still relevant, they need to be respected \eqref{N7}.

\subsection{Modelling with same-day transfers \ref{lp:SDTransfer}}\label{sec:SDTransfer}
In general, allowing no transfers at all quickly renders instances infeasible or leads to solutions with very low objective value for $\privobj$.
One slight but effective generalisation is to allow transfers only for patients arriving in the current first time period.
% In this case, we use the same variables as in model \eqref{lp:noTransfer} and minimise additionally the total number of reassignments, i.e., \begin{align*}    \min\quad \transobj = \sum_{(p,r)\in \rpold} \sum_{r' \in \R\setminus\{r\}}x_{pr'} \end{align*} instead of fixing the previous assignments \eqref{N7}.\textbf{O\R:}
In this case, we use the same variables as in model \eqref{lp:noTransfer} and maximise the total number of not reassigned present patients, i.e.,
\begin{align*}
    \gamma^* := \max\quad \left(\transobj = \sum_{(p,r)\in \rpold} x_{pr}\right)
\end{align*}
instead of fixing the previous assignments \eqref{N7}.
Remark that here the total number of transfers is given by $|\rpold|-\gamma^*$. 
We then obtain the IP model \eqref{lp:SDTransfer}, which is given in \cref{app:lpC}. 

\subsection{IP-formulation with arbitrary many transfers \ref{lp:allTransfer}}\label{sec:IParbTrans}
Finally, we provide an IP model where transfers are allowed in between all time periods and we minimise the total number of transfers.
We use variables $x_{prt}\in\{0,1\}$ which denote that at time-interval $t\in \T$, patient $p\in \P$ is assigned to room $r\in \R$ and variables $\delta_{prt}\in\{0,1\}$ that account whether patient $p$ is transferred from room $r$ to another room between time periods $t$ and $t+1$, i.e.,
\begin{align*}
x_{prt}&=\begin{cases}
            1,  &\text{if patient }  p \text{ is assigned to room } r \text{ in time period } t,\\
            0,  &\text{otherwise,}
        \end{cases}\\
\delta_{prt}&=\begin{cases}
            1,  &\text{if }  \ass(p,t)=r,~ \ass(p,t)\neq r \text{ and } \arr_p \leq t < \dis_p -1,\\
            0,  &\text{otherwise,}
        \end{cases}    
\end{align*}
as well as variables $g_{rt}, s_{prt}\in\{0,1\}$ as before.
The total number of transfers is then computed as
\[
    \transobj=\sum_{p\in \P}\sum_{t=\arr_p}^{\dis_p-1}\sum_{r\in \R} \delta_{prt}
\]
and we employ the following integer programming formulation:
\beforeMyLP{4}
\begin{maxi!}
{}{(\privobj,-\transobj)\label{E0}}{\label{lp:allTransfer}}{}
\addConstraint{\sum_{r \in \R} x_{prt}}{= 1\label{E1}}{\forall t\in \T, p \in \P(t)}
\addConstraint{\sum_{p \in \fp(t)} x_{prt} + \sum_{\tiny p \in \fp(t) \cap \priv} (c_r-1)s_{prt}}{\le c_rg_{rt}\label{E2}}{\forall t \in \T, r \in \R}
\addConstraint{\sum_{p \in \mp(t)} x_{prt} + \sum_{p \in \mp(t) \cap \priv} (c_r-1)s_{prt}}{\le c_r(1-g_{rt})\; \label{E3}}{\forall t \in \T, r \in \R}
\addConstraint{s_{prt}}{\le x_{prt}\label{E5}}{\forall t \in \T,  r \in \R, p \in \priv}
\addConstraint{x_{prt}+x_{qrt}}{\le 1\label{E6}}{\forall r \in \R,(p,q) \in \conflicts,t \in \T}
\addConstraint{x_{prt}-x_{pr(t+1)}}{\le \delta_{prt}\label{E7}}{\forall p \in \P, \arr_p \leq t < \dis_p -2, r \in \R}
\addConstraint{x_{prt},g_{rt},s_{prt},\delta_{prt}}{\in \{0,1\} \notag{}}{\forall r \in \R, t \in \T, p \in \P.}
\end{maxi!}
\afterMyLP

Here, we ensure that every patient receives a bed via \eqref{E1}.
Constraints \eqref{E2}, and respectively \eqref{E3}, ensure on the one hand that every double-bed room only contains only either female or male patients up to its capacity, an, on the other hand, they record when a private patient is alone in a double-bed room.
The constraints \eqref{E5} link the single room variables $s_{prt}$ to the patient
assignments and \eqref{E6} ensures that all patient conflicts are respected.
Finally, constraints \eqref{E7} ensure that all transfers are accounted for.

\subsubsection{Objective Cuts}\label{sec:objcuts}
If we know the exact value of $\smax_t$, as discussed in \cref{sec:dualBounds}, we can use  constraints of the type\begin{align*} \label{B} \tag{B} 
\sum_{\substack{p \in \priv(t)}} s_{prt} \le \smax_t \quad \forall t \in \T
\end{align*}
to help the solver.
The valid inequalities defined in \ref{B} are indeed cutting planes. For that consider the following example with four patients and three double rooms.

\todo{restructure using subfigures and state corresponding values of LP-variables}
\begin{figure}[ht!]
\centering

\scalebox{0.35}{
\begin{tikzpicture}[node distance=2cm,every label/.style={align=left}]

\tikzstyle male=[fill=green!20];
\tikzstyle female=[fill=blue!20];
\tikzstyle fixed=[line width=2mm];
\tikzstyle privatepartner=[pattern=north west lines, pattern color=black];

draw=black,->

% 1st Layer

% Room 1
\draw[dashed,fill=gray!20] (0,0) rectangle (6,3);
\draw[female] (0.5,0.5) rectangle (2.5,2.5) node[pos=.5] {\huge F1};
\draw[male] (3.5,0.5) rectangle (5.5,2.5) node[pos=.5] {\huge M1};

% Room 2
\draw[dashed] (7,0) rectangle (13,3);
\draw[female] (7.5,0.5) rectangle (9.5,2.5) node[pos=.5] {\huge F2};
\draw[privatepartner] (10.5,0.5) rectangle (12.5,2.5) node[pos=.5] {};

% Room 3
\draw[dashed] (14,0) rectangle (20,3);
\draw[male] (14.5,0.5) rectangle (16.5,2.5) node[pos=.5] {\huge M2};
\draw[privatepartner] (17.5,0.5) rectangle (19.5,2.5) node[pos=.5] {};

% Inbetween

\node (text1) at (10,-0.8) {\huge The upper assignment is feasible and optimal in the LP relaxation.};

% 2nd Layer (-4.5)

\draw[dashed,fill=gray!20] (0,-4.5) rectangle (6,-1.5);
\draw[male] (0.5,-4) rectangle (2.5,-2) node[pos=.5] {\huge M1};
\draw[male] (3.5,-4) rectangle (5.5,-2) node[pos=.5] {\huge M2};

% Room 2
\draw[dashed] (7,-4.5) rectangle (13,-1.5);
\draw[female] (7.5,-4) rectangle (9.5,-2) node[pos=.5] {\huge F2};
\draw[privatepartner] (10.5,-4) rectangle (12.5,-2) node[pos=.5] {};

% Room 3
\draw[dashed] (14,-4.5) rectangle (20,-1.5);
\draw[female] (14.5,-4) rectangle (16.5,-2) node[pos=.5] {\huge F1};
\draw[] (17.5,-4) rectangle (19.5,-2) node[pos=.5] {};
\end{tikzpicture}}
    
    \caption{Shaded beds are kept free for private patients. The patients F2, M2 are private patients and the patients F1, M1 are regular patients.}
    \label{fig:lpgap}
\end{figure}
Here we have two male and two female patients, one of who is a private patient each. By violating integrality on $g_{rt}$ in the first room, we can assign two private patient beds this time period. Since this results in a higher objective value, branching on $g_{rt}$ is needed to ensure sex separation. Furthermore, for symmetric rooms the solver will simply permute the patient assignment through the rooms until branching has been performed on sufficiently many $g_{rt}$ variables. Note that the above empirically significantly outperforms a standard $$x_{prt}\le g_{prt} \;\;\forall p \in \P, r\in \R, t \in \T $$model extension, as shown in \cref{sec:objcutsdiscussion}.

\subsubsection{Properties of the IP formulations}\label{sec:integrality}\todo{new}
\todo{clarify goal of this section}
Although it is arguable to make general statements about the hardness of solving IPs for a given formulation, there are several promising facts about the formulations introduced here. First, all variables are all binary. Second, the constraint matrix only contains coefficients from $-1,0,1, ... , c_r-1$, which simplifies to $-1,0,1$ for double rooms, ensuring numerical stability. 

Clearly, $g$ does not need to be integral and indeed, optimal solutions for the LP relaxation will have fractional values for $g$ as this removes the need to respect sex separation. Based on this, we can calculate an upper bound on the value of the LP relaxation of \ref{lp:noTransfer}/\ref{lp:SDTransfer}.

\begin{lemma}
\todo{choose more readable variable name than $\smax_{t,frac}$}
For feasible instances with $\rc_r\in\{1,2\}$, the maximum fractional number $\smax_{t,frac}$ of private patients who can get a room for themselves in time period $t\in \T$ if sex separation is violated can be computed via
\begin{align*}
\smax_{t,frac} = \min \left\{\abs{\priv(t)},2\abs{\R}-\abs{\P(t)}\right\} 
\end{align*}
\end{lemma}
\begin{proof} Let $c^* \coloneqq \abs{\{r \in \R : c_r = 1\}}$ be the number of single rooms. If there are more single rooms $c^*$ than private patients, the above follows immediately. Else, $c^*$ private patients get a single room and $\abs{\priv(t)}-c^*$ private patients remain. Each of those can get a single room iff there is a free bed to match with them. If sex separation can be ignored, the number of free beds is given by $2(\abs{\R}-c^*)-(\abs{\P(t)}-c^*)=2\abs{\R}-\abs{\P(t)}-c^*$. This results in
\begin{align*}
    &c^* + \min \left\{\abs{\priv(t)}-c^*,2\abs{\R}-\abs{\P(t)}-c^*\right\}\\
    = &\min \left\{\abs{\priv(t)},2\abs{\R}-\abs{\P(t)}\right\}
\end{align*}
private patient single rooms. The above also holds for $\priv\le c^*$, which concludes the proof.
\end{proof}

This implies that the absolute LP-gap can be bounded a priori. Note that this does not apply for the relative LP gap, which can be arbitrary large, as illustrated in Figure \ref{fig:rellpgap}.
\todo{restructure using subfigures and state corresponding values of LP-variables}
\begin{figure}[ht!]
\centering

\scalebox{0.35}{
\begin{tikzpicture}[node distance=2cm,every label/.style={align=left}]

\tikzstyle male=[fill=green!20];
\tikzstyle female=[fill=blue!20];
\tikzstyle fixed=[line width=2mm];
\tikzstyle privatepartner=[pattern=north west lines, pattern color=black];

draw=black,->

% 1st Layer

% Room 1
\draw[dashed,fill=gray!20] (0,0) rectangle (6,3);
\draw[female] (0.5,0.5) rectangle (2.5,2.5) node[pos=.5] {\huge F1};
\draw[male] (3.5,0.5) rectangle (5.5,2.5) node[pos=.5] {\huge M1};

% Room 2
\draw[dashed] (7,0) rectangle (10,3);
\draw[female] (7.5,0.5) rectangle (9.5,2.5) node[pos=.5] {\huge F2};
% Inbetween

\node (text1) at (5,-0.8) {\huge The upper assignment is feasible and optimal in the LP relaxation.};

% 2nd Layer (-4.5)

\draw[dashed,fill=gray!20] (0,-4.5) rectangle (6,-1.5);
\draw[female] (0.5,-4) rectangle (2.5,-2) node[pos=.5] {\huge F1};
\draw[female] (3.5,-4) rectangle (5.5,-2) node[pos=.5] {\huge F2};

% Room 2
\draw[dashed] (7,-4.5) rectangle (10,-1.5);
\draw[male] (7.5,-4) rectangle (9.5,-2) node[pos=.5] {\huge M1};

\end{tikzpicture}}
    \caption{The private patient F2 only gets a single room in the fractional LP relaxation. F1, M1 are regular patients.}
    \label{fig:rellpgap}
\end{figure}

In comparison, for the absolute gap we find that:
\begin{lemma}
For feasible instances with $\rc_r\in\{1,2\}$ it holds that
\begin{align*}
        \smax_{t,frac} - \smax_t \in \{0,1\}
\end{align*}
for any time period $t\in \T$.
\end{lemma}
\begin{proof}
We consider the three cases for $s_t^{max}$ separately. Let first $\alpha_t \geq \abs{\priv(t)}$ then by definition
\begin{align*}
&\abs{\R}-\frac{\abs{\P(t)\setminus \priv}}{2} 
=\, \abs{\R}-\frac{\abs{\fp(t)\setminus \priv}}{2} - \frac{\abs{\mp(t)\setminus\priv}}{2} \\
\ge\, &\abs{\R}-\ceil*{\frac{\abs{\fp(t)\setminus \priv}}{2}} - \ceil*{\frac{\abs{\mp(t)\setminus\priv}}{2}} = \alpha_t \ge \abs{\priv(t)}\\
\implies\,& 2\abs{\R}-\abs{\P(t)} \ge \abs{\priv(t)}
\end{align*}
and therefore $\smax_{t,frac} = \smax_t = \abs{\priv(t)}.$ 

Now let $\alpha_t = \abs{\priv(t)}-1 \text{ and } \beta^\mathrm{f}_t=\beta^\mathrm{m}_t=1$, i.e., the number of male and female non-private patients is odd and there is at least on male and female private patient.
In this case, the exact solution contains $\abs{\priv(t)}-1$ private patient places and w.l.o.g. there must be a male private patient in a double room with a male non-private patient and a female non-private patient in a room without a roommate. By putting the male and female non-private patient together, we can achieve $\smax_{t,frac}=\abs{\priv(t)}$ in the fractional solution.

Finally, let $\alpha_t < \abs{\priv(t)}-1$. In the exact solution we then have 
\begin{align*}
\smax_{t}&=2\alpha_t + \beta^\mathrm{f}_t + \beta^\mathrm{m}_t - \abs{\priv(t)}\\
&=2\abs{\R}-2\ceil*{\frac{\abs{\fp(t)\setminus \priv}}{2}} - 2\ceil*{\frac{\abs{\mp(t)\setminus\priv}}{2}}+\beta^\mathrm{f}_t + \beta^\mathrm{m}_t - \abs{\priv(t)}
\end{align*}
W.l.o.g. consider the term
$$- 2\ceil*{\frac{\abs{\fp(t)\setminus\priv}}{2}}+\underbrace{\min\left\{\abs{\fp(t)\setminus \priv}\mod{2},~\abs{\fp(t)\cap \priv}\right\}}_{\beta^\mathrm{f}_t}.$$
If $\abs{\fp(t)\setminus \priv}$ is even, the latter  becomes zero and the former reduces to $-\abs{\fp(t)\setminus \priv}$. If $\abs{\fp(t)\setminus \priv}$ is odd then $\beta^\mathrm{f}_t$ becomes one and the former term reduces to $-\abs{\fp(t)\setminus \priv}-1$. In either case the total is $-\abs{\fp(t)\setminus \priv}$. In either case:
\begin{align*}
\smax_{t}&=2\abs{\R}-\abs{\mp(t)\setminus \priv} -\abs{\fp(t)\setminus \priv}- \abs{\priv(t)}\\
&= 2\abs{\R}-\abs{\P(t)\setminus \priv}-\abs{\priv(t)}=2\abs{\R}-\abs{\P(t)}.
\end{align*}
Since $\alpha_t < \abs{\priv(t)}-1$ this is also smaller than $\abs{\priv(t)}$ and therefore $\smax_{t,frac} = \smax_t = 2\abs{\R}-\abs{\P(t)}.$
\end{proof}
